# Supplementary material for: Probabilistic 3d regression with projected huber distribution
Source: arXiv:2303.05245 source file (2023-03-09)
Supplement: Supplementary file 1 [file supp_moments.tex]

\label{sec:supp_moments}
Here we derive the moments up to the second moment.

\begin{align}
E\begin{bmatrix}
x/z \\ y/z
\end{bmatrix} &= \mu_p\\
Var\begin{bmatrix}
x/z \\ y/z
\end{bmatrix} &\propto A^{-1}A^{-1} \dfrac {(\Gamma(-2/a,1) + \Gamma(2/a,1))} {2\Gamma(0,1)} \\
E\left[z \right] &= \dfrac {\Gamma(1/a,1) + \Gamma(-1/a,1)} {2\Gamma(0,1)} \mu_z\\
Var\left[z \right] &= \dfrac {2\Gamma(0,1)(\Gamma(2/a,1) + \Gamma(-2/a,1)) - (\Gamma(1/a,1)+\Gamma(-1/a,1))^2} {4\Gamma(0,1)^2} \mu_z^2\\
E\left[log(z) \right] &= \mu_z \\
Var\left[log(z) \right] &\propto 1/a^2
\end{align}

In practice, for the allowed values for $a$ the Gamma fraction range between $1$ to $1.28$ for the expression determining $Var[x/z, y/z]$.
The expected value of $z$ is $\mu_z$ adjusted by an expression of a. The gamma term for $E[z]$ range between 1.07 and 1.0, for the allowed range of $a$. \textit{the analytical formula of the variance is quite hard to parse.}

\textbf{Proof of projected coordinates}

For this proof we will use the notation
\begin{equation}
v_p = \begin{bmatrix}
x/z \\ y/z
\end{bmatrix}
\end{equation}
This is slightly different than the notation in the rest of the work

\begin{align}
E\begin{bmatrix}
x/z \\ y/z
\end{bmatrix} &= \dfrac{1} {K(A, \mu, a)}
    \int \begin{bmatrix}
x/z \\ y/z
\end{bmatrix} \exp\left(-h\left(\left\|A\begin{bmatrix} x/z-\mu_x \\ y/z-\mu_y \end{bmatrix}\right\|_2\dfrac{z}{\mu_z}\right)
    - \log(z/\mu_z) - \exp(a|\log(z/\mu_z)|)\right) dxdydz \\
&= \mu_p + \dfrac {1} {(2\Gamma(0,1))(1+\exp(-1/2))} \int\limits_{-\infty}^{\infty} \exp(-s/a) A^{-1}\int\limits_{\mathbb{R}^2} q \exp(-h(\|q\|_2))dq\exp(-\exp(|s|))ds \\
&= \mu_p
\end{align} 

The first step is doing the same basis change as equation \ref{eq:basis_change_norm_factor_1} and \ref{eq:basis_change_norm_factor_2} with
\begin{equation}
v_p = \mu_p + A^{-1}q\dfrac{z} {\mu_z}
\end{equation}

Since $\mu_p$ is does not depend on the variables we integrate over we know the expected value of it is itself.

The second step is realizing that the distribution is symmetric with respect to $q$. Therefore the expected value of $q$ is 0.

We now compute 
\begin{align}
    Var\left[v_p\right] &= E\left[v_p v_p^T\right] - E\left[v_p\right] E\left[v_p^T\right] \\
    &= E\left[\mu_p \mu_p^T + \mu_p q^TA^{-1}z\mu_z + A^{-1}q\mu_z^Tz\mu_z + A^{-1}qq^TA^{-1}\dfrac{z^2}{\mu_z^2}\right] - \mu_p \mu_p^T \\
    &= E\left[A^{-1}qq^TA^{-1}\exp(2s/a)\right] \\ 
    &= A^{-1}E\left[qq^T\exp(2s/a)\right]A^{-1}
\end{align}

\begin{align}
    E\left[qq^T\exp(2s/a)\right]
    &= \dfrac {1}{K(A,\mu,a)} \int\limits_{0}^{\infty} \int\limits_{\mathbb{R}^2} qq^T\exp(-h(\|q\|))dq \exp(2s/a) \exp(-\exp(|s|))ds \\
    &= \dfrac {I} {2\pi(2\Gamma(0,1))(1+\exp(-1/2))}
    \int\limits_{0}^{\infty}\int\limits_{0}^{2\pi} r^3\cos^2(\theta) \exp(-h(r)) d\theta dr \\
    & (\int\limits_{0}^{\infty} \exp(-2s/a -\exp(s))ds + \int\limits_{0}^{\infty} \exp(2s/a -\exp(s))ds) \\
    &= I \dfrac {\pi(13\exp(-1/2)+2)(\Gamma(-2/a, 1) + \Gamma(2/a, 1))} {2\pi(2\Gamma(0,1))(1+\exp(-1/2))} \\
    &= I \dfrac {(13\exp(-1/2)+2)(\Gamma(-2/a, 1) + \Gamma(2/a, 1))} {2(2\Gamma(0,1))(1+\exp(-1/2))}
\end{align}

Putting this together with the computation for the variance concludes the proof.

\textbf{proof of expected z coordinate}

First note $z = \exp(s/a)\mu_z$
\begin{align}
E\left[z\right] &= \dfrac {\int\limits_{\infty}^{\infty} \exp(s/a-\exp(|s|))\mu_z} {\int\limits_{\infty}^{\infty} \exp(\exp(|s|))} \\
&= \dfrac {\Gamma(1/a,1)+\Gamma(-1/a,1)} {2\Gamma(0,1)}\mu_z
\end{align}

\begin{align}
E\left[z^2\right] &= \dfrac {\int\limits_{\infty}^{\infty} \exp(2s/a-\exp(|s|))\mu_z^2} {\int\limits_{\infty}^{\infty} \exp(\exp(|s|))} \\
&= \dfrac {\Gamma(2/a,1)+\Gamma(-2/a,1)} {2\Gamma(0,1)}\mu_z^2
\end{align}
Which gives
