# Supplementary material for: Probabilistic 3d regression with projected huber distribution
Source: arXiv:2303.05245 source file (2023-03-09)
Supplement: Supplementary file 2 [file supp_constraint_2.tex]

TODO
