# Supplementary material for: Probabilistic 3d regression with projected huber distribution
Source: arXiv:2303.05245 source file (2023-03-09)
Supplement: Supplementary file 3 [file supp_proof_basis_change.tex]

In this section we prove that the negative log likelihood of 
equation \ref{eq:norm_factor_prob} result in equation \ref{eq:loss_after_basis_change} after the parameter change in \ref{eqs:basis_change_variables} and \ref{eqs:basis_change_parameters}

We state these equations for reference

\begin{equation}
    p(x,y,z) = \dfrac{1} {K(A, \mu, a)} \exp(-h\left(\left\|A\begin{bmatrix} x/z-\mu_x \\ y/z-\mu_y \end{bmatrix}\right\|_2\dfrac{z}{\mu_z}\right) - \log(z/\mu_z) - \exp(h(a|\log(z/\mu_z)|)))
\end{equation}

\begin{align}
    v_p = \begin{bmatrix} x_p \\ y_p \end{bmatrix} &= \begin{bmatrix} \dfrac{2fx} {zS} \\ \dfrac{2fy} {zS} \end{bmatrix} \\  
    z_p &= \log\left(\dfrac{zS} {\mu_{z0}f}\right) / D \\ 
    b &= a*D \\
    \nu_v = \begin{bmatrix} \nu_x \\ \nu_y \end{bmatrix} &= \dfrac {f\mu_{z0}} {S\mu_z} A \begin{bmatrix} \mu_x \\ \mu_y \end{bmatrix} \\
    \nu_z &= a\log\left(\dfrac {\mu_zS} {\mu_{z0}f}\right) \\
    B &= \dfrac {A\mu_{z0}} {2\mu_z} 
\end{align}

The negative log likelihood with the original parameterization turns into

\begin{align}
\label{eq:loss_orig_basis_term_1}
    L(x,y,z;A,a,\mu) &= h\left(\left\|A\begin{bmatrix} x/z-\mu_x \\ y/z-\mu_y \end{bmatrix}\right\|_2\dfrac{z}{\mu_z}\right) \\
    \label{eq:loss_orig_basis_term_2}
    &+ \exp(h(a|\log(z/\mu_z)|)) \\
    \label{eq:loss_orig_basis_term_log_z_mu}
    &+ \log(z/\mu_z) \\
    &+ \log(K(A, \mu, a))
\end{align}

The term \ref{eq:loss_orig_basis_term_1} becomes

\begin{align}
&h\left(\left\|A\begin{bmatrix} x/z-\mu_x \\ y/z-\mu_y \end{bmatrix}\right\|_2\dfrac {z}{\mu_z}\right) = \\
&= h\left(\left\|A\begin{bmatrix} x/z \\ y/z \end{bmatrix}\ \dfrac{z} {\mu_z}- A\begin{bmatrix} \mu_x \\ \mu_y \end{bmatrix} \dfrac{z} {\mu_z} \right\|_2\right) = \\
&= h\left(\left\|\dfrac {2B\mu_z} {\mu_{z,0}} \dfrac{S}{2f}\begin{bmatrix} x_p \\ y_p \end{bmatrix} \dfrac{\exp(z_pD)f\mu_{z,0}} {S\mu_z} - \dfrac{\nu_v S \mu_z} {f \mu_{z,0}} \dfrac {f\mu_{z,0}} {S\mu_z} \exp(z_pD) \right\|_2\right) = \\
&= h\left(\left\|Bv_p-\nu_v\right\|_2\exp(z_pD)\right)
\end{align}

The term \ref{eq:loss_orig_basis_term_2} becomes

\begin{align}
\exp(h(a\log(z/\mu_z))) &= \exp(h\left(a \log\left(\dfrac{\exp^{z_pD} \dfrac {\mu_{z,0}f} {S}} {\exp^{\nu_z/a} \dfrac {\mu_{z,0}f} {S}}\right) \right)) \\
&= \exp(h(a(z_pD-\nu_z/a))) \\
&= \exp(h(bz_p-\nu_z))
\end{align}

From section \ref{sec:deriving_normalizing_factor} we know that the normalizing factor is 


\begin{equation}
K(A, \mu, a) = \dfrac {\mu_z^3} {|A|a}C_{norm\_constant}   
\end{equation}

therefore
\begin{align}
\label{eq:NLL_norm_factor}
\log(K(A, \mu, a)) &= 3\log(\mu_z) - \log(|A|) - \log(a) + \log(C_{norm\_constant}) \\
&= \log(\mu_z) - \log(|A\mu_{z0}/2\mu_z|) + 2\log(\mu_{z0}) - 2\log(2) - \log(aD) + \log(D) + log(C_{norm\_constant}) \\
&= \log(\mu_z) - \log(|B|) + 2\log(\mu_{z0}) - 2\log(2) - \log(b) + \log(D) + log(C_{norm\_constant})
\end{align}

We notice how the $\log(\mu_z)$ term will turn the term $\log(z/\mu_z)$ in equation \ref{eq:loss_orig_basis_term_log_z_mu} into $log(z)$.

here $log(C_{norm\_constant}$ swallows terms related to $S, f, \mu_{z,0},D$. The term $\log(\mu_z)$ will cancel out $\mu_z$ in $\log(z/\mu_z)$

In addition the variable change from $x,y,z$ to $x_p, y_p, z_p$ introduces a scale change corresponding to
\begin{align}
dv_p &= \dfrac{dv} {\begin{vmatrix}
  \dfrac{\partial x} {\partial x_p} & \dfrac{\partial x} {\partial y_p} & \dfrac{\partial x} {\partial z_p} \\
  \dfrac{\partial y} {\partial x_p} & \dfrac{\partial y} {\partial y_p} & \dfrac{\partial y} {\partial z_p} \\
  \dfrac{\partial z} {\partial x_p} & \dfrac{\partial z} {\partial y_p} & \dfrac{\partial z} {\partial z_p}
  \end{vmatrix}} \\
  &= \dfrac{dv} {\begin{vmatrix}
  2f/zS & 0 & -2fx/z^2S \\
  0 & 2f/zS & -2fy/z^2S \\
  0 & 0 & Dz \\
  \end{vmatrix}} \\
  &= \dfrac{ S^2zD} {4f^2}dv
\end{align}

This factor will result in the term
\begin{align}
   -\log{\dfrac{ S^2zD} {4f^2}} &= - \log(z) - \log{\dfrac{D S^2} {4f^2}}
\end{align}
in the loss. The $-log(z)$ term will cancel out $log(z)$ part of $log(z/\mu_z)$ in equation \ref{eq:loss_orig_basis_term_log_z_mu}, Since the $\mu_z$ part of the term was already canceled out by $\log(K(B, \nu, b))$ the $log(z/\mu_z)$ term is now completely canceled out. The other terms are constants for each sample and will not contribute to the gradients when training. Thus we can consider them part of $C_{norm\_constant}$ when analyzing the loss.

Adding the terms together yields equation \ref{eq:loss_after_basis_change}, concluding the proof.
